# Supplementary material for: Orientational order of motile defects in active nematics
Source: arXiv:1501.06228 ancillary file (2015-07-09)
Supplement: Supplementary file 1 [file supplement.pdf]

# Orientational Order of Motile Defects in Active Nematics Supplementary Materials

Stephen J. DeCamp[1*], Gabriel S. Redner[1*], Aparna Baskaran[1], Michael F. Hagan[1] & Zvonimir Dogic[1]

[1] *Department of Physics, Brandeis University, Waltham MA 02454, USA*

[*] *These authors contributed equally to the work*

# Table of Contents

1. Supplementary Figures
2. Supplementary Videos
3. Distribution of Bend and Splay
4. Experimental Methods
5. Simulation Methods
6. Defect Detection and Tracking
7. Simulation Rod Length Distribution
8. Error Estimation for Fig. 3b
9. Calculation of Noise Floor in Figs. 3a, b

# 1: Supplementary Figures

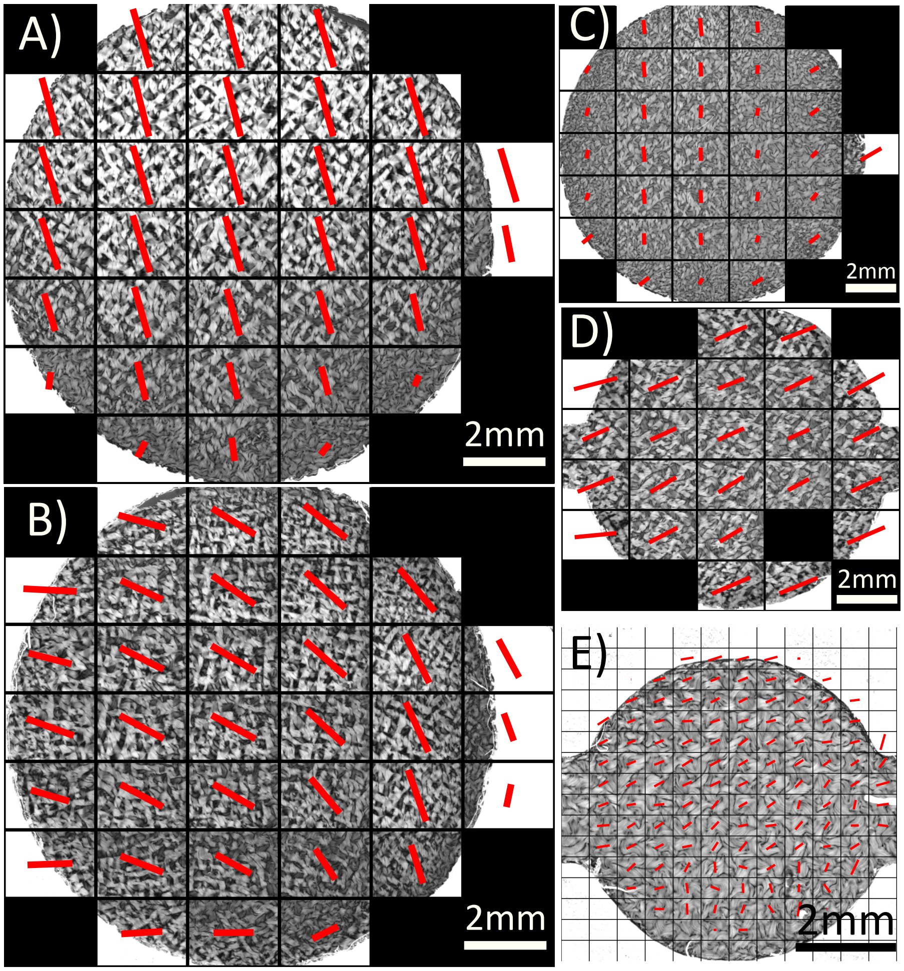


**Supplementary Figure 1: Defect alignment is independent of boundary conditions.** Retardance maps from several active nematic experiments in circular chambers. The red bar in each box indicates the preferred axis computed from $+1/2$ defects within that box, and its length is proportional to the degree of local order. Circles in panels A-D are 10mm in diameter while E is 6mm in diameter. In all cases, MT films form defect-ordered phases with a single system-spanning preferred axis.

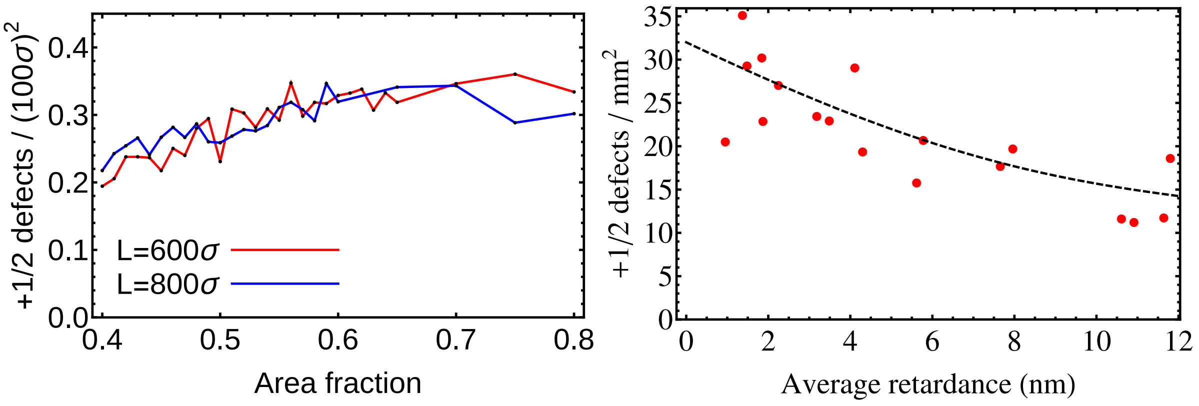


**Supplementary Figure 2: Density of defects.** Left: Mean density of +1/2 defects in simulations of box size $600\sigma \times 600\sigma$ and $800\sigma \times 800\sigma$ as a function of overall rod area fraction. Right: mean density of +1/2 defects in experiments as a function of retardance. In simulations the defect density increases weakly with overall system density, while in experiments it decreases weakly. A number of factors may account for this difference, including the fact that our simulations are purely 2D, while the MT film in experiments can thicken in the third dimension.

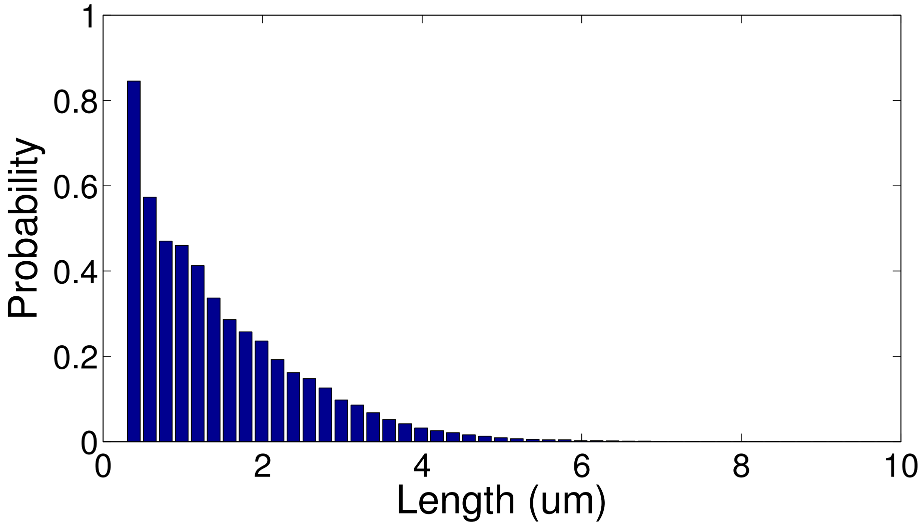


**Supplementary Figure 3: Microtubule length distribution.** The mean length of microtubule filaments in the experiments is measured to be 1.3um. This is determined by depleting filaments onto clean microscope glass using a 6% Dextran solution in M2B buffer so they lay in the imaging plane. The microtubules are imaged with a 100x objective and lengths are measured using IDL image processing.

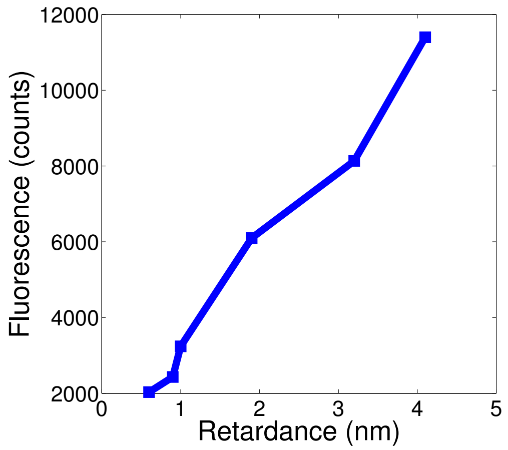


**Supplementary Figure 4: Retardance and fluorescence measurements are proportional.** It has been measured that birefringence increases linearly with the number of MTs in a bundle[1]. As the MT nematic is composed of bundles with near-perfect local alignment, the retardance ($\langle\Delta\rangle$ = thickness $\times$ birefringence) effectively reports the thickness of the sample. We confirm this by checking that the fluorescence, which directly measures the amount of material present in the sample, varies roughly linearly with the retardance of the sample. We note that the 3D packing fraction of MTs within the quasi-2D film is not directly measurable by these methods.

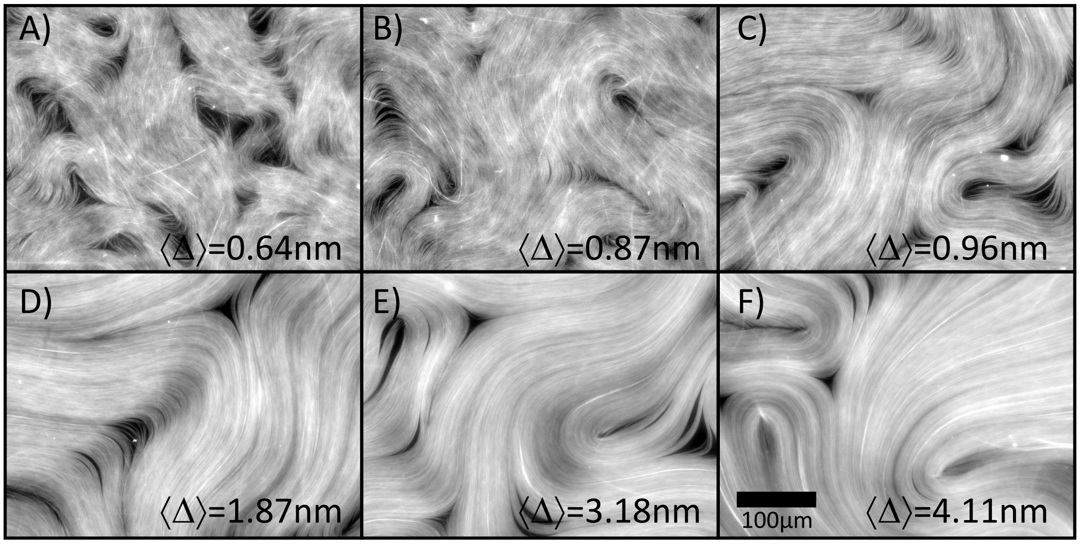


**Supplementary Figure 5: MT film morphology changes with system density.** Here, we show representative snapshots of samples for a series of retardance values ($\langle\Delta\rangle$). The scale bar in F applies to all panels.

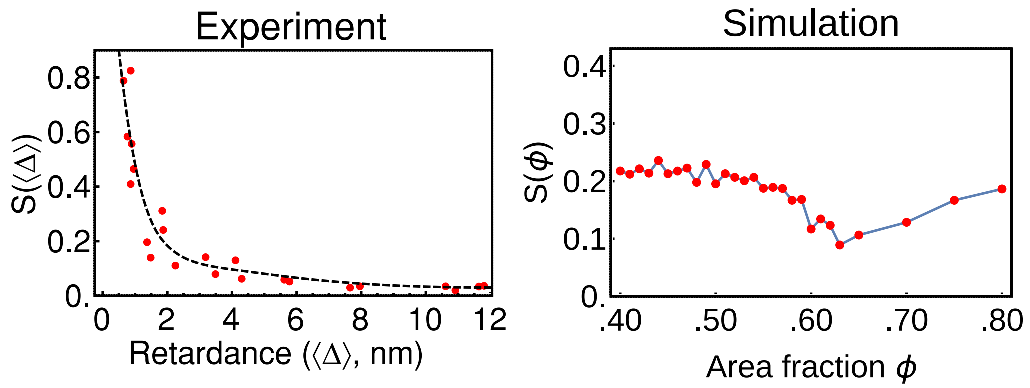


**Supplementary Figure 6: Nematic order of underlying MTs/rods.** Nematic order parameter $S$ computed from the configurations of the underlying microtubules (left) and simulated rods (right), as a function of system density. The degree of nematic order of the rods follows the degree of ordering of defects (Fig. 3A, B in the main text). We believe that the rise in $S(\phi)$ at high area fraction is a finite-size artifact.

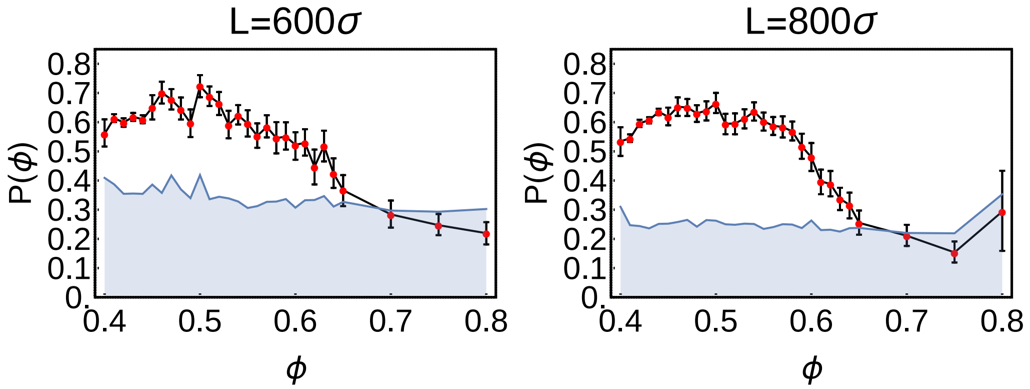


**Supplementary Figure 7: Nematic order of underlying MTs/rods.** Polar defect order parameter $P(\phi)$ for systems of size $600\sigma \times 600\sigma$ (left) and $800\sigma \times 800\sigma$ (right). The transition appears to sharpen as the system size is increased.

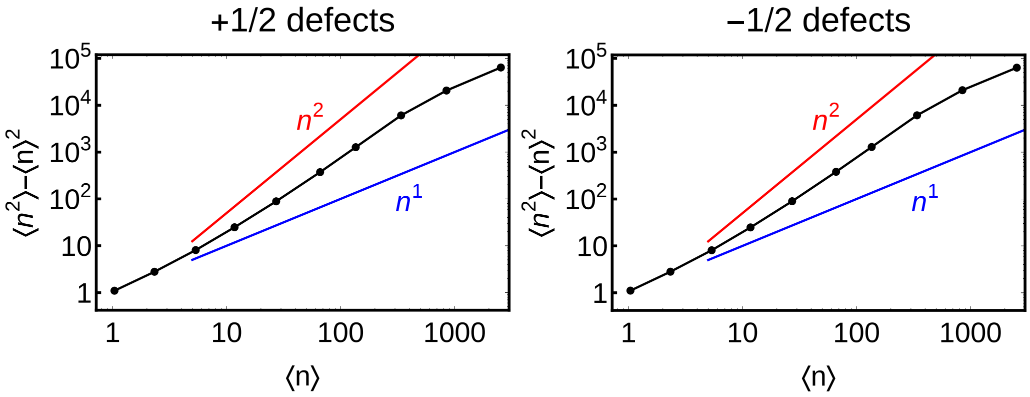


**Supplementary Figure 8: Giant number fluctuations of defects.** Both +1/2 and -1/2 defects display giant density fluctuations in a large experimental system ($2 \times 6$ cm, containing roughly $20,000$ defects). We plot here the mean and variance of defect counts in subsystems of various sizes, showing the variance growing much faster than the mean, as is common in many active systems.

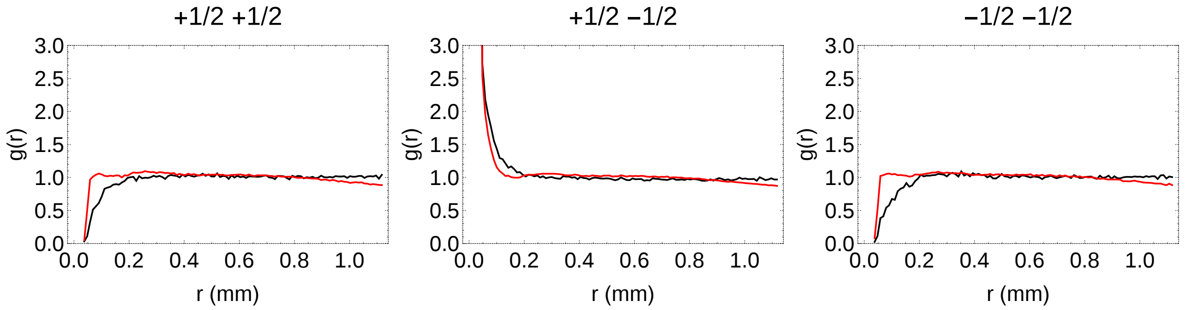


**Supplementary Figure 9: Spatial correlations between defects in experiments.** Spatial pair correlation function $g(r)$ for defect positions in experimental systems. As above, three measurements are shown; left, for +1/2 defects exclusively, center, for pairs of +1/2 and -1/2 defects, and right, for -1/2 defects exclusively. Again, no appreciable structure is observed beyond the first peak. The black plots are for an isotropic system with $\langle \Delta \rangle = 10.61\,\text{nm}$, while the red plots are for a defect-ordered system with $\langle \Delta \rangle = 0.89\,\text{nm}$.

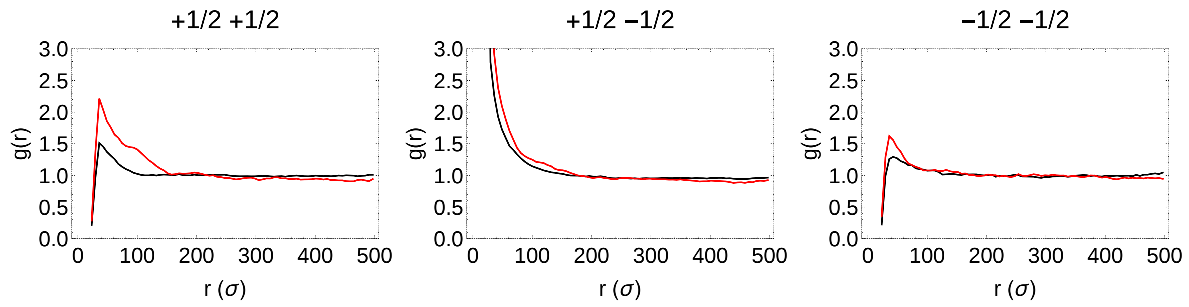


**Supplementary Figure 10: Spatial correlations between defects in simulations.** These plots show the spatial pair correlation function $g(r)$ for defect positions in simulation systems. Three measurements are shown; left, for +1/2 defects exclusively, center, for pairs of +1/2 and -1/2 defects, and right, for -1/2 defects exclusively. It is clear that +1/2 and -1/2 defects repel at short distances, while $\pm 1/2$ pairs are frequently found at small separations, such as immediately after creation, or just before annihilation. In all cases, no appreciable structure is observed beyond the first peak. The black plots are for isotropic systems with $\phi = 0.70$, while the red plots are for defect-ordered systems with $\phi = 0.50$.

# 2: Supplementary Videos

## Supplementary Video 1: 2D Active Nematic Under Fluorescence Microscopy

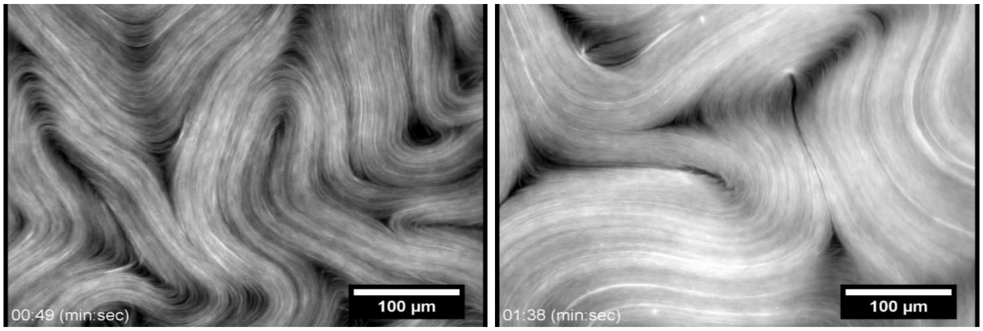


Using fluorescence microscopy, we visualize an extensile active nematic which is composed of microtubule filaments and kinesin motor proteins which are confined at a 2D, flat oil-water interface. $\pm 1/2$ defects stream across the nematic and are spontaneously created and annihilated at equal rates in the steady state. Here, the fluorescence videos for a high and a low retardance sample are shown.

## Supplementary Video 2: Retardance Video of 2D Active Nematic

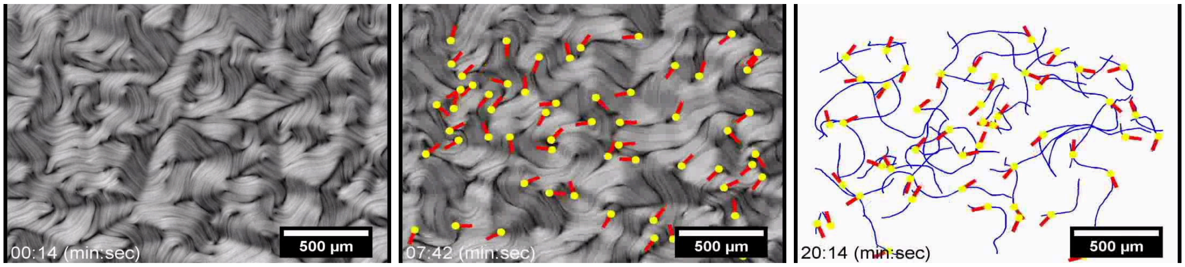


Retardance images taken with LC-PolScope provide a quantitative spatial map of birefringence in the active nematic. Here, a large field of view shows many $\pm 1/2$ defects streaming across the sample. The results of our defect tracking algorithm are then overlaid onto the retardance image. Yellow dots indicate $+1/2$ defect positions, and red lines indicate the orientations of

their fracture lines. The defect markers are then shown on a white background for clarity. Finally, we show the tracks of $+1/2$ defect trajectories in blue.

## Supplementary Video 3: Large-Scale Orientation of Defects

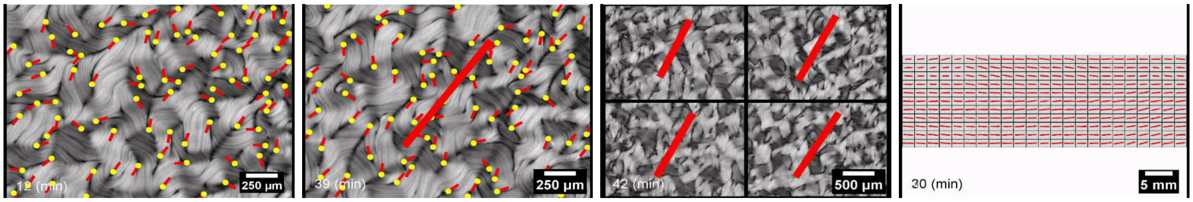


Retardance images taken with LC-PolScope show defect configurations in an MT sample. First, positions and orientations of $+1/2$ defects in a single FOV (2.2mm $\times$ 1.7mm) are shown. The average orientation axis of the $+1/2$ defects is then depicted by the orientation of a red line in the center of the FOV. This axis is then shown persisting across multiple fields of view. Finally, the orientation axis is shown across a very large sample (5.1cm $\times$ 1.9cm), showing that the direction of defect alignment spans the entire macroscopic sample.

## Supplementary Video 4: Simulated 2D Active Nematic in Isotropic Phase

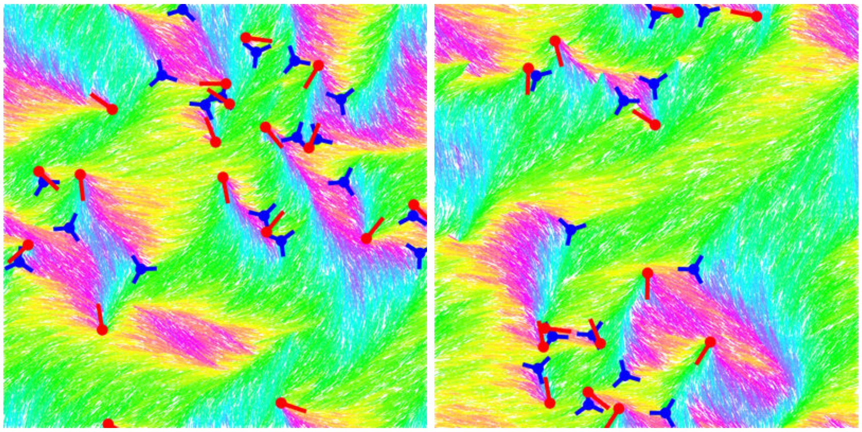

Simulation of an active nematic with area fraction $\phi = 0.75$, showing +1/2 defects pointing chaotically in all directions. The size of the simulation box is $800\sigma \times 800\sigma$, where $\sigma$ is the width of a single rod.

## Supplementary Video 5: Simulated 2D Active Nematic in Polar Phase

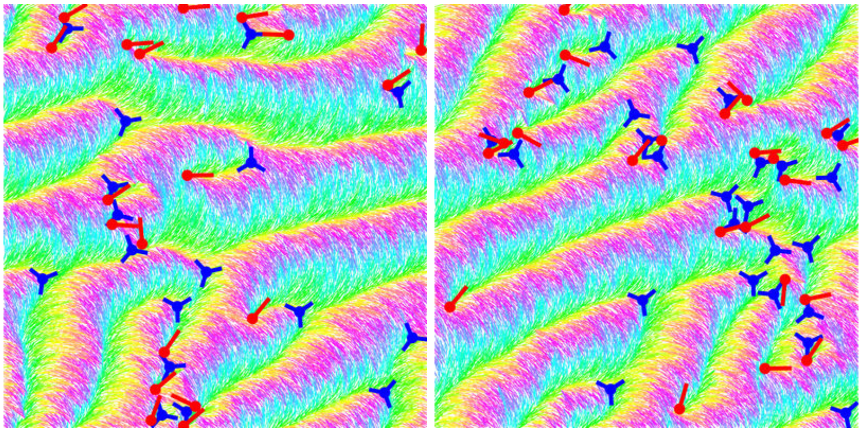

Simulation with area fraction $\phi = 0.55$, showing strong polar alignment of +1/2 defects which travel through the system, leaving aligned structures in the nematic field. The size of the simulation box is $800\sigma \times 800\sigma$, where $\sigma$ is the width of a single rod.

# 3: Distribution of Bend and Splay

In equilibrium 2D nematics, the Frank free energy density is:

$$f(\boldsymbol{r}) = \frac{K_1}{2}(\nabla \cdot \hat{\boldsymbol{n}})^2 + \frac{K_3}{2}(\hat{\boldsymbol{n}} \times \nabla \times \hat{\boldsymbol{n}})^2 \tag{1}$$

Here $K_1$ is the splay constant and $K_3$ is the bend constant. Given a coarse-grained director field computed from LC-PolScope output or a simulation frame, we can calculate the density of bend and splay distortion at each point in the sample, which can reveal otherwise-hidden information about the sample's structure.

Here, we represent the magnitude of bend (splay) deformation at each pixel by the intensity of the green (red) channel. The intensity scale is the same for the two types of deformation.

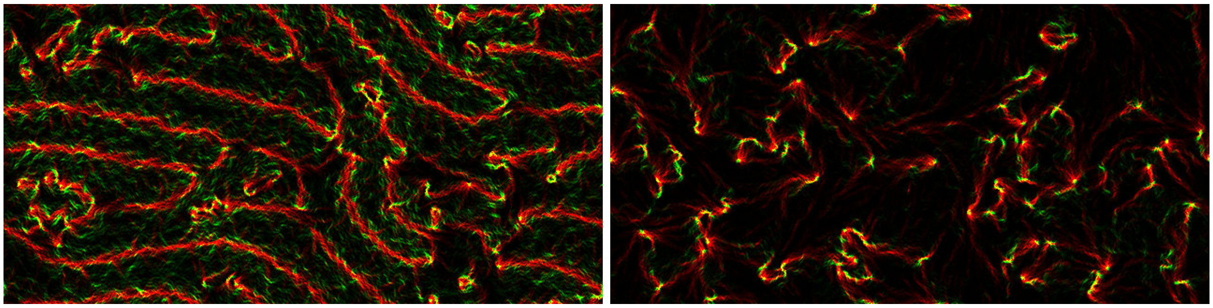

The left image represents a system in the polar phase with $\phi = 0.55$, while the system on the right is isotropic with $\phi = 0.70$. In both systems, bend is mostly concentrated in the vicinity of defects, while splay is localized along linear structures which stretch through the system. In the polar phase these structures align along the direction of defect ordering, while in the isotropic phase they are disordered. There is also less distortion overall in the high-density system, in which the bend and splay constants are higher[2].

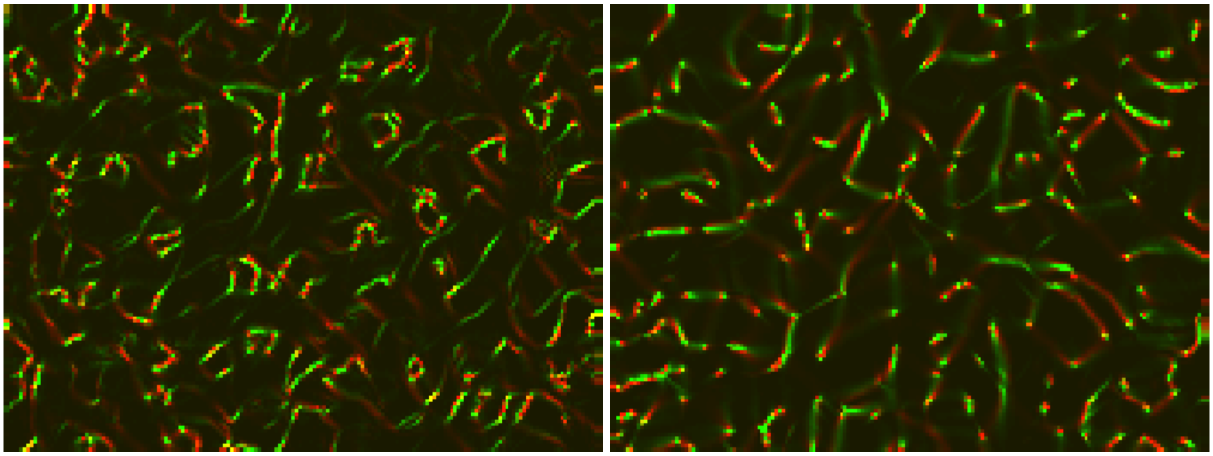

On the left we have the bend and splay values for one FOV of an experimental system in the nematic phase with $\langle\Delta\rangle = 0.33$ nm. On the right is a system in the isotropic phase with $\langle\Delta\rangle = 2.81$ nm. In both, we see that neither bend nor splay is dominant, and both are distributed along linear structures which do not exhibit obvious alignment. Though the length-scales of features clearly differ between the two images, it is not otherwise clear how to identify defect-ordered states from bend and splay distributions in experiments.

# 4: Experimental Methods

We purified tubulin from bovine brain using two polymerization/depolymerization cycles in high molarity PIPES buffer[3]. Tubulin was labeled with NHS-ester Alexa 647 (Life Technologies A-20006) using previously published protocols[4]. Microtubules were formed by co-polymerizing labeled tubulin and unlabeled tubulin with non-hydrolayzalbe analog of GTP, Guanosine-5-[($\alpha, \beta$)-methyleno]triphosphate (GMPCPP) (Jena Bioscience NU-405L). The final labeled fraction of tubulin monomers is 3%. Polymerization with GMPCPP generates shorter MT filaments than with Taxol stabilization, and they have an average length of 1.3 $\mu$m. Similar to Taxol stabilized microtubules, those stabilized with GMPCCP do not exhibit any monomer turnover.

The kinesin motor protein is the 401-amino acid N-terminal domain from Drosophila melanogaster fused to the *E. coli* Biotin Carboxyl Carrier Protein (BCCP) and labeled with a six Histidine tag[5]. K401-bio-6HIS are expressed in *E. coli* and purified on a nickel column. They were then dialyzed against 50mM Imidozole, frozen in a 20% sucrose solution, and stored at -80 C.

Motor clusters were formed by incubating purified kinesin motor proteins with tetrameric streptavidin in a stoichiometric ratio of about two motors per one streptavidin for 30 minutes while on ice.

Active pre-mixtures were created by combining kinesin motor clusters, ATP, an ATP regeneration system composed of phosphoenol pyruvate (PEP) and pyruvate kinase/lactic dehydrogenase (PK/LDH), the depletion agent polyethylene glycol (PEG), an anti-oxidant system based on glucose oxidase, catylase, glucose, and Trolox to prevent photo-bleaching[6]. All components are finally diluted to working concentrations with the microtubule buffer (M2B). Before use, microtubules are combined with the active pre-mixture. The fuel regeneration system ensures that any ADP produced by kinesin hydrolysis is immediately recycled into ATP. These regeneration protocols can power active nematics for over 24 hours, ensuring a constant ATP concentration throughout the experiment.

To make large, flat 2D active nematics, microscope slide glass is incubated with Aquapel for 1 minute and then sonicated in DI water for 5 minutes to create a fluorophilic surface. Cover glass is coated with poly-acrylamide to create a passive, hydrophilic surface[7]. Flow cells of arbitrarily large sizes are made by applying 100$\mu$m thick, laser-cut, double-sided transfer tape (3M 93005LE) to the microscope glass slide and applying the cover slip to the top surface of the tape. In order to create the flat oil-water interface, the flow cell is flooded with HFE-7500 oil with 1.8% Fluoro-Surfactant (RAN Biotechnologies) immediately followed by flowing in the water phase containing the active microtubule mixture while simultaneously wicking out the oil. A thin film of oil, approximately 1-4$\mu$m thick, is left coating the Aquapel glass. Slides are

then put in a Sorval Legend RT (rotor #6434) centrifuge for 4 minutes at 1000RPM to quickly sediment the microtubule bundles to the oil-water interface, and hasten the formation of the quasi-2D nematic film. This procedure ensures that there are no filaments in the bulk of the flow cell.

Imaging the active microtubule nematic is done using conventional fluorescence microscopy with a Nikon Ti Eclipse and an Andor Clara camera running open-source microscopy managing software micromanager. Information regarding the nematic director field and the retardance of the nematic is gathered using LC-PolScope microscopy which consists of a set of electronically controlled active cross-polarizers from which the director orientation and retardance are computed using a 5-frame acquisition algorithm[8]. Using LC-PolScope to collect global birefringence information leads to spatial distortions in the retardance maps that are not easily corrected by local retardance background subtraction techniques. These distortions (at low retardance values) are manifest as alternating dark/light regions in nematic retardance map and occurs when the local birefringence in the microscope glass constructively/destructively reinforces the birefringence of the sample.

# 5: Simulation Methods

The system's state is represented by the center-of-mass positions, orientations, and lengths $\{\boldsymbol{r}_i, \theta_i, L_i\}_{i=1}^N$ of the rods. Their spatial dynamics are governed by the coupled overdamped Langevin equations:

$$\dot{\boldsymbol{r}}_i = \Xi_i^{-1} \cdot \boldsymbol{F}_i + \boldsymbol{\eta}_{i,\mathrm{T}} \tag{2}$$

$$\dot{\theta}_i = \gamma_{i,R}^{-1} T_i + \eta_{i,\mathrm{R}} \tag{3}$$

Here $\boldsymbol{F}_i$ and $T_i$ represent the systematic force and torque on rod $i$. The friction coefficients[9] are:

$$\Xi_i = \gamma_{i,\parallel} \hat{\boldsymbol{u}}_i \hat{\boldsymbol{u}}_i + \gamma_{i,\perp} (\boldsymbol{I} - \hat{\boldsymbol{u}}_i \hat{\boldsymbol{u}}_i) \tag{4}$$

$$\gamma_{i,\parallel} = \frac{2\pi\mu L_i}{\ln(L_i/\sigma)} \quad \gamma_{i,\perp} = 2\gamma_{i,\parallel} \quad \gamma_{i,\mathrm{R}} = \frac{L_i^2}{6}\gamma_{i,\parallel} \tag{5}$$

with $\hat{\boldsymbol{u}}_i = (\cos\theta_i, \sin\theta_i)$ and $\boldsymbol{I}$ the unit tensor. The $\eta$ represent Gaussian white noise variables with $\langle \eta(t) \rangle = 0$, $\langle \eta_i(t) \eta_j(t') \rangle = 0$, and:

$$\langle \boldsymbol{\eta}_{i,\mathrm{T}}(t) \boldsymbol{\eta}_{i,\mathrm{T}}(t') \rangle = 2k_\mathrm{B} T \Xi_i^{-1} \delta(t - t') \tag{6}$$

$$\langle \eta_{i,\mathrm{R}}(t) \eta_{i,\mathrm{R}}(t') \rangle = 2k_\mathrm{B} T \gamma_{i,R}^{-1} \delta(t - t') \tag{7}$$

Rods interact via a WCA potential acting between the points of closest approach[10]:

$$V_\mathrm{WCA} = 4\left[\left(\frac{\sigma}{r}\right)^{12} - \left(\frac{\sigma}{r}\right)^{6}\right] + 1 \quad \text{if} \quad r < 2^{(1/6)}\sigma \quad \text{and 0 otherwise} \tag{8}$$

The extension of rods is governed by:

$$\dot{L}_i = v_\mathrm{ex} \tag{9}$$

When the rod length exceeds $L_\mathrm{max} = 21\sigma$, it is removed from the simulation and replaced by two shorter rods. New rod lengths are chosen such that $L_1 + L_2 = L_\mathrm{max}$. However, since

splitting rods exactly in half would eventually lead to synchronization of splitting times across the whole simulation, we instead select $L_1$ by drawing randomly from a uniform distribution between $9\sigma$ and $12\sigma$. In steady-state, these dynamics lead to a nontrivial distribution of rod lengths, described in detail in a later section.

In the same timestep as a rod is split, another rod is eliminated elsewhere in the simulation to keep the number of particles fixed. This rod is selected by searching system-wide for the pair of rods whose centers of mass are closest, and selecting one of the pair. This models the longitudinal merging of bundles, and has the side-effect of suppressing the giant number fluctuations[11,12] and phase separation[13] which are characteristic of many active nematics, but do not appear in the MT system.

We nondimensionalized the equations of motion using the spherocylinder width $\sigma$ and $k_{\mathrm{B}}T$ as basic units of length and energy, and $\tau = \frac{\sigma^2}{D_0} = \frac{3\pi\mu\sigma^3}{k_{\mathrm{B}}T}$ as the unit of time, where $D_0$ is the diffusion constant of a sphere of radius $\sigma$, and $\mu$ is the viscosity of the Brownian solvent. Simulations employed the stochastic Runge-Kutta method[14] with an adaptive time step of maximum value $5 \times 10^{-}5\tau$. The simulations in this study were performed with $v_{\mathrm{ex}} = 80\frac{\sigma}{\tau}$.

# 6: Defect Detection and Tracking

Defect processing occurs in three phases: detection, orientation measurement, and tracking.

The defect detection algorithm[15] works by choosing a trial point, and selecting the orientations of all rods or pixels within a fixed distance $r_{\text{max}}$ (20 pixels for experiments, corresponding to 32.25 $\mu$m, or $20\sigma$ for simulations). The selected data are split into eight wedges about the trial point, and the average director for each octant is calculated. The rotation of these directions about the center point, if nonzero, indicates the presence and strength of a defect. This procedure is repeated at a large number of trial points ($\sim 6500$ for a single microscope FOV, or 1600 for an $800\sigma \times 800\sigma$ simulation box). A multi-stage mesh refinement scheme selects additional points for testing in the vicinity of already-detected defects. A clustering algorithm groups these points, and the centroid of each cluster is taken as the location of the defect.

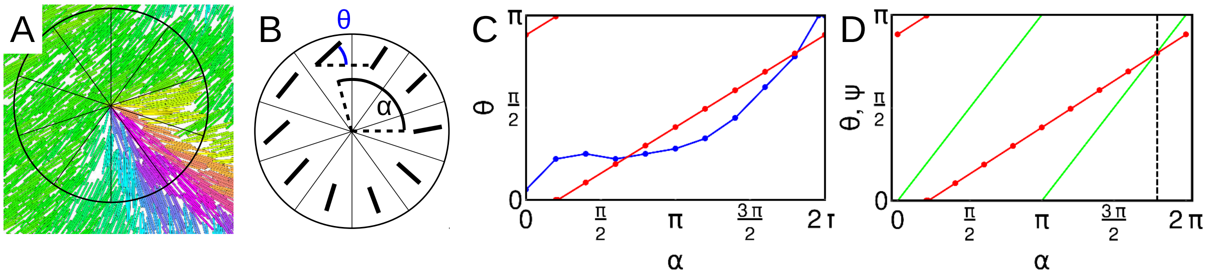


The procedure for detecting the orientation of a +1/2 defect is illustrated here. First, we select all rods (or LC-PolScope pixels) within $r_{\text{max}}$ of the defect core, divide them into ten wedges (A), and calculate the average orientation $\theta$ in each wedge (B). The results are parametrized by the angle $\alpha$ that the center of the wedge makes with respect the defect core. The resulting function $\theta(\alpha)$ (blue) is then smoothed (red) (C). We then locate the point at which $\theta(\alpha) = \alpha + n\pi$ (green) is found (black dashed line) (D); in other words, where the nematogens are pointing along an axis passing through the defect core. For +1/2 defects, this selects the direction pointing along the "comet tail".

To handle the threefold symmetry of -1/2 defects, we reduce the angles $\alpha$ of all rods or LC-PolScope pixels modulo $\frac{2\pi}{3}$, and then proceed as above.

Defect trajectories are calculated by employing a tracking algorithm originally used for tracking colloidal particles under video microscopy[16] to the locations of +1/2 and -1/2 defects separately. In equilibrium colloids, the cost function used when evaluating inter-frame particle motion is a Gaussian, which is justified because colloidal particles move diffusively. In our nonequilibrium system, it is unclear *a priori* what the cost function should be. In practice, we find that a cost function which is linear in defects' inter-frame displacements works well.

# 7: Simulation Rod Length Distribution

Due to the complex dynamics of rod growth and division, the steady-state distribution of their lengths is nontrivial. Knowledge of this distribution is necessary at several points, such as when selecting the number of rods to achieve a given steady-state area fraction. In this section we derive this distribution.

## Evenly-Split Rods

In our simulations, rods are not split directly in half, in order to avoid synchronization of splitting times across the system. However, the derivation of the rod length distribution is considerably simpler in the case of equally-split rods. We therefore show this derivation first to demonstrate our techniques, before presenting the general case.

We represent the time-dependent rod length probability distribution by $b(\ell, t)$. Its evolution is governed by:

$$\frac{\partial b}{\partial t} = -v_{\text{ex}} \frac{\partial b}{\partial \ell} - \kappa b \tag{10}$$

Here $v_{\text{ex}}$ is the extension rate of the rods, and $\kappa$ is the rate at which rods are randomly eliminated. These two rates are related, but we treat them as independent constants for now.

The general solution to the evolution equation is:

$$b(\ell, t) = c(t) e^{-\frac{\kappa \ell}{v_{\text{ex}}}} \left( t - \frac{\ell}{v_{\text{ex}}} \right) \tag{11}$$

The constant $c(t)$ is determined by normalization. Denoting by $\ell_1$ and $\ell_2$ the lengths of rods when they are created and destroyed, we obtain:

$$\frac{1}{c(t)} = \int_{\ell_1}^{\ell_2} e^{-\frac{\kappa \ell}{v_{\text{ex}}}} \left( t - \frac{\ell}{v_{\text{ex}}} \right) \tag{12}$$

Integrating and taking the limit $t \to \infty$, we find the general steady-state form for $b(\ell)$:

$$b(\ell) = \frac{e^{-\frac{k\ell}{v_{\text{ex}}}} \kappa}{\left( e^{-\frac{k\ell_1}{v_{\text{ex}}}} - e^{-\frac{k\ell_2}{v_{\text{ex}}}} \right) v_{\text{ex}}} \tag{13}$$

We next determine the relationship between $\kappa$ and $v_{\text{ex}}$. In a timeslice $dt$, the number of rods which reach the maximum size is $N v_{\text{ex}} b(\ell_2) dt$, where $N$ is the total number of rods in the system. Since the number of rods eliminated in a time period is the same as the number which reach the maximum size, we have $\kappa = v_{\text{ex}} b(\ell_2)$, or:

$$\frac{\kappa}{v_{\text{ex}}} = \frac{\ln 2}{\ell_2 - \ell_1} \tag{14}$$

Additionally, we have $\ell_1 = \ell_2/2$. Plugging in, we find the steady-state rod length PDF $b(\ell)$ and CDF $B(\ell)$ are then:

$$b(\ell) = \frac{8 \ln 2}{2^{\frac{2\ell}{\ell_2}} \ell_2} \qquad B(\ell) = 2\left(1 - \frac{2}{2^{\frac{2\ell}{\ell_2}}}\right) \tag{15}$$

Plugging in the values used in simulation ($\ell_2 = 21\sigma$), we can visualize these distributions:

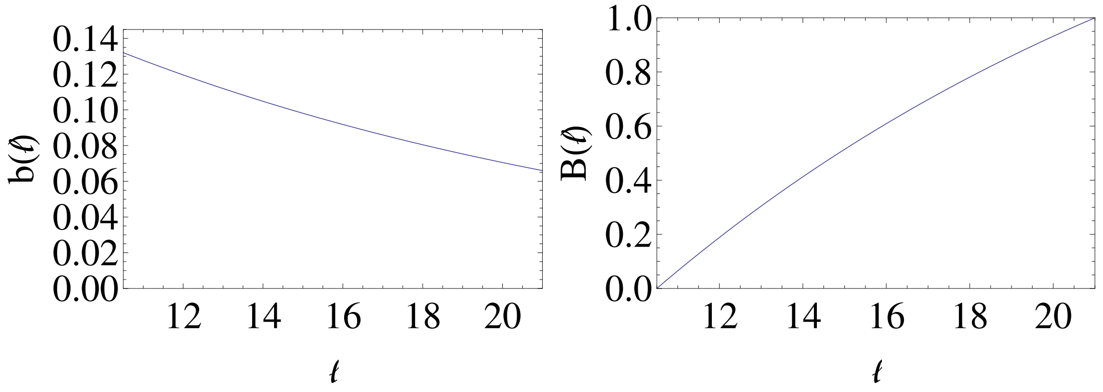


The mean rod length is:

$$\langle \ell \rangle = \frac{\ell_2}{\ln 4} \approx 15.14\sigma \tag{16}$$

## Unevenly-Split Rods

In our simulations, the point at which to split a rod is selected from a uniform distribution with a small range about its midpoint. The rod length distribution is more complex to derive in this case, and requires a minor approximation.

Once again, our goal is to calculate $b(\ell, t)$. We have three lengths to contend with: $\ell_2$ is the length at which a rod is split. $\ell_0$ and $\ell_1$ are the minimum and maximum lengths of the fragments

which can be created when a long rod is split ($9\sigma$ and $12\sigma$ respectively in our simulations). We denote by I the region between $\ell_0$ and $\ell_1$, and by II the region between $\ell_1$ and $\ell_2$.

The evolution of $b(\ell, t)$ in region II is the same as in the previous section. In region I, its evolution has an extra term due to the creation of new rods. The evolution equations are:

$$\begin{aligned}
\mathrm{I}: \quad & \frac{\partial b_{\mathrm{I}}}{\partial t} = -v_{\mathrm{ex}} \frac{\partial b_{\mathrm{I}}}{\partial \ell} - \kappa b_{\mathrm{I}} + 2\kappa \frac{\ell_2 - \ell_0}{\ell_1 - \ell_0} \\
\mathrm{II}: \quad & \frac{\partial b_{\mathrm{II}}}{\partial t} = -v_{\mathrm{ex}} \frac{\partial b_{\mathrm{II}}}{\partial \ell} - \kappa b_{\mathrm{II}}
\end{aligned}$$

In region I, we additionally have the constraint that $b(\ell_0, t) = 0$. The general solutions are:

$$\begin{aligned}
\mathrm{I}: \quad & b_{\mathrm{I}}(\ell, t) = c_0 \left(1 - e^{\frac{\kappa}{v_{\mathrm{ex}}}(\ell_0 - \ell)}\right) \frac{\ell_2 - \ell_0}{\ell_1 - \ell_0} \\
\mathrm{II}: \quad & b_{\mathrm{II}}(\ell, t) = c_0 c_1(t) e^{-\frac{\kappa \ell}{v_{\mathrm{ex}}}} \left(t - \frac{\ell}{v_{\mathrm{ex}}}\right)
\end{aligned}$$

We determine $c_1$ by enforcing that $b(\ell, t)$ is continuous at $\ell = \ell_2$:

$$c_1(t) = \left(e^{\frac{\kappa \ell_1}{v_{\mathrm{ex}}}} - e^{\frac{\kappa \ell_0}{v_{\mathrm{ex}}}}\right) \frac{\ell_2 - \ell_0}{\ell_1 - \ell_0} \left(\frac{v_{\mathrm{ex}}}{\ell_1 - t v_{\mathrm{ex}}}\right)$$

We determine $c_0$ by normalization:

$$\frac{1}{c_0} = \kappa(\ell_2 - \ell_0) + \frac{v_{\mathrm{ex}}}{\kappa} e^{-\frac{\kappa \ell_2}{v_{\mathrm{ex}}}} \left(e^{\frac{\kappa \ell_0}{v_{\mathrm{ex}}}} - e^{\frac{\kappa \ell_1}{v_{\mathrm{ex}}}}\right)$$

The probability distribution is then:

$$\begin{aligned}
\mathrm{I}: \quad & b_{\mathrm{I}}(\ell) = z \left(e^{\frac{\kappa(2\ell - \ell_2 + 2p)}{2 v_{\mathrm{ex}}}} - 1\right) \\
\mathrm{II}: \quad & b_{\mathrm{II}}(\ell) = z \left(e^{\frac{2\kappa p}{v_{\mathrm{ex}}}} - 1\right) \\
& \text{with} \quad z = \frac{\kappa e^{\frac{\kappa(\ell_2 - \ell)}{v_{\mathrm{ex}}}}}{2\kappa p e^{\frac{\kappa(\ell_2 + 2p)}{2 v_{\mathrm{ex}}}} + v_{\mathrm{ex}} \left(1 - e^{\frac{2\kappa p}{v_{\mathrm{ex}}}}\right)}
\end{aligned}$$

with $p = (\ell_1 - \ell_0)/2$. The next step should be to determine the relationship between $v_{\text{ex}}$ and $\kappa$. However, the resulting equation is transcendental and cannot be solved directly. Instead we assume that the ratio $\frac{\kappa}{v_{\text{ex}}} = \lambda$ is the same as in the equal-length splitting case: $\lambda_0 = \frac{\log 4}{\ell_2}$, which turns out to be a surprisingly good approximation. To demonstrate this, we numerically solve the equation $\lambda = b(\ell_2)$, and compare the result to $\lambda_0$. For the values used in simulation, we find $\lambda_0 \approx 0.066014$ and $\lambda = b(\ell_2) \approx 0.663202$, giving a relative error of only $0.33\%$. This error is negligible, so we assign $\lambda = \lambda_0$ at this point.

We now insert $\frac{\kappa}{v_{\text{ex}}} = \frac{\log 4}{\ell_2}$ to find the full probability distribution which depends on $\ell_2$ and $p$ only:

$$\text{I}: \quad b_{\text{I}}(\ell) = \left(2^{1-\frac{2\ell}{\ell_2}} - 2^{\frac{2p}{\ell_2}}\right) \left[\frac{4 \ln 2}{\left(2^{\frac{4p}{\ell_2}} - 1\right)\ell_2 - 2^{3+\frac{2p}{\ell_2}} p \ln 2}\right]$$

$$\text{II}: \quad b_{\text{II}}(\ell) = 2^{1-\frac{2\ell}{\ell_2}} \left(1 - 2^{\frac{4p}{\ell_2}}\right) \left[\frac{4 \ln 2}{\left(2^{\frac{4p}{\ell_2}} - 1\right)\ell_2 - 2^{3+\frac{2p}{\ell_2}} p \ln 2}\right]$$

The cumulative distribution is:

$$\text{I}: \quad B_{\text{I}}(\ell) = \left(-2^{2-\frac{2\ell}{\ell_2}} + 2^{1+\frac{2p}{\ell_2}} \left(\ell_2 + (\ell_2 - 2\ell - 2p)\ln 2\right)\right) \left[\frac{1}{\left(2^{\frac{4p}{\ell_2}} - 1\right)\ell_2 - 2^{3+\frac{2p}{\ell_2}} p \ln 2}\right]$$

$$\text{II}: \quad B_{\text{II}}(\ell) = \left(2^{2-\frac{2\ell}{\ell_2}} \left(\ell_2 - 2^{\frac{4p}{\ell_2}}\ell_2 + 2^{1+\frac{2(\ell+p)}{\ell_2}} p \ln 2\right)\right) \left[\frac{1}{\left(2^{\frac{4p}{\ell_2}} - 1\right)\ell_2 - 2^{3+\frac{2p}{\ell_2}} p \ln 2}\right]$$

The probability distributions look like:

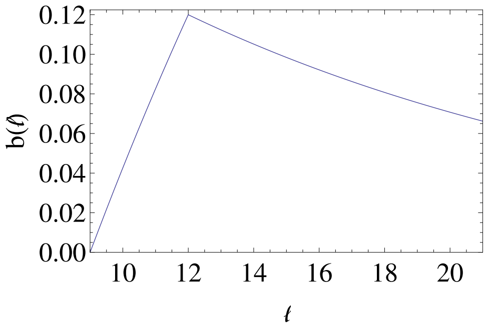


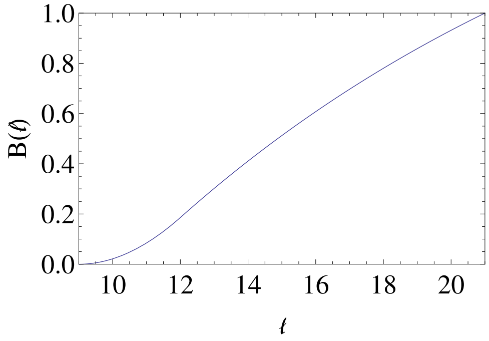

The mean rod length is:

$$\langle \ell \rangle = \ell_2 + \frac{\ell_2}{\ln 4} + \frac{2^{2+\frac{2p}{\ell_2}} \ell_2 p \ln 2}{\ell_2 \left(2^{\frac{4p}{\ell_2}} - 1\right) - 2^{3+\frac{2p}{\ell_2}} p \ln 2} \approx 15.11$$

## 8: Error Estimation for Fig. 3b

At each area fraction value, we have trajectories from several simulations (approximately 10) with defects located and tracked. In each trajectory, we first calculate the polar order parameter $P$ for each frame, and then compute the normalized autocorrelation function of this time-series. We estimate the correlation time by finding the time at which this function first falls below $e^{-1}$. We then select a subset of frames from the trajectory such that they are spaced at least twice this far apart in time. This procedure produces a set of minimally-correlated system configurations for one trajectory. After applying this decimation procedure to each trajectory, we combine all of the resulting frames into one pool.

Since we cannot easily model or propagate errors through this procedure, we turn to bootstrap methods. For each area fraction for which we are producing a data point for the figure, we follow this procedure:

- For N (number of bootstrap samples) = 1 to 500:
  - For each of the uncorrelated sample frames:
    - Select a synthetic data set by sampling with replacement from the defect orientations in that frame
    - Calculate the order parameter $P$ for this synthetic data
  - Average these measurements to get $\langle P \rangle$ for the synthetic data
- Sort the list of resulting $\langle P \rangle$ measurements. The $0.25N$th and $0.95N$th elements of this list represent the bounds of the 90% confidence region for this data point.

# 9: Calculation of Noise Floor in Figs. 3a, b

The blue-tinted "noise floor" which appears in Figs. 3A and 3B marks the 95% confidence interval for the measurement of $\langle P \rangle$ if the defect data were drawn from a perfectly-isotropic uniform distribution. It is computed by the following procedure:

- For N (number of bootstrap samples) = 1 to 500:
  - For each of the uncorrelated sample frames
    - Generate a random data set by sampling from a uniform distribution on the range $[0, 2\pi]$ with the same number of samples as there are defects in the sample frame
    - Calculate the order parameter $P$ for this synthetic data
  - Average these measurements to get $\langle P \rangle$ for the synthetic data
- Sort the list of resulting $\langle P \rangle$ measurements. The $0.95N$th element of this list represents the maximum bound of the 95% confidence region for an isotropic sample containing the same number and combination of data points as the real sample.

1. Oldenbourg, R., Salmon, E. D. & Tran, P. T. Birefringence of single and bundled microtubules. *Biophysical journal* **74**, 645–654 (1998).

2. Allen, M. & Frenkel, D. Calculation of liquid-crystal Frank constants by computer simulation. *Physical Review A* **37**, 1813 (1988).

3. Castoldi, M. & Popov, A. V. Purification of brain tubulin through two cycles of polymerization-depolymerization in a high-molarity buffer. *Protein expression and purification* **32**, 83 (2003).

4. Hyman, A. *et al.* Preparation of modified tubulins. *Methods in enzymology* **196**, 478 (1991).

5. Subramanian, R. & Gelles, J. Two distinct modes of processive kinesin movement in mixtures of ATP and AMP-PNP. *The Journal of general physiology* **130**, 445 (2007).

6. Sanchez, T. & Dogic, Z. Engineering oscillating microtubule bundles. *Methods in Enzymology* **524**, 205 (2013).

7. Lau, A. W. C., Prasad, A. & Dogic, Z. Condensation of isolated semi-flexible filaments driven by depletion interactions. *EPL (Europhysics Letters)* **87**, 48006 (2009).

8. Shribak, M. & Oldenbourg, R. Techniques for Fast and Sensitive Measurements of Two-Dimensional Birefringence Distributions. *Applied Optics* **42**, 3009 (2003).

9. Tao, Y.-G., den Otter, W. K., Padding, J. T., Dhont, J. K. G. & Briels, W. J. Brownian dynamics simulations of the self- and collective rotational diffusion coefficients of rigid long thin rods. *The Journal of chemical physics* **122**, 244903 (2005).

10. McCandlish, S. R., Baskaran, A. & Hagan, M. F. Spontaneous segregation of self-propelled particles with different motilities. *Soft Matter* **8**, 2527 (2012).

11. Ramaswamy, S., Simha, R. A. & Toner, J. Active nematics on a substrate: Giant number fluctuations and long-time tails. *Europhysics Letters (EPL)* **62**, 196 (2003).

12. Narayan, V., Ramaswamy, S. & Menon, N. Long-lived giant number fluctuations in a swarming granular nematic. *Science* **317**, 105 (2007).

13. Mishra, S. & Ramaswamy, S. Active Nematics Are Intrinsically Phase Separated. *Physical Review Letters* **97**, 090602 (2006).

14. Brańka, A. & Heyes, D. Algorithms for Brownian dynamics computer simulations: Multivariable case. *Physical Review E* **60**, 2381 (1999).

15. Bates, M. A. Nematic ordering and defects on the surface of a sphere: a Monte Carlo simulation study. *The Journal of chemical physics* **128**, 104707 (2008).

16. Crocker, J. Methods of Digital Video Microscopy for Colloidal Studies. *Journal of Colloid and Interface Science* **179**, 298 (1996).
